# Supplementary material for: Attention-Driven Training-Free Efficiency Enhancement of Diffusion Models
Source: arXiv:2405.05252 source file (2024-05-08)
Supplement: Supplementary file 1 [file X_suppl_old.tex]

\clearpage
\setcounter{page}{1}
\maketitlesupplementary
\appendix

\section{Profile of FLOPs, Latency, and Parameters}
\label{app:profile}

To validate the conclusion that the sampling cost dominates generation cost and the cost of attention layers dominates the sampling cost, we investigate the FLOPs, latency, and parameter breakdown for different diffusion backbones.

\subsection{Stable Diffusion Models}

%The overall architecture of SDM is demonstrated in Fig.\ref{fig:sdm}. 

The key difference between SDM and previous DMs is that it relies on training of a variational autoencoder (VAE) to encode the pixel space into the latent space and employs the DM in the latent space, which reduces computational cost significantly. 

% \begin{figure}[t]
%   \centering
%    \includegraphics[width=\linewidth]{sec/SDM.png}

%    \caption{The general architecture of Stable Diffusion Models. Figure adapted from [13]}
%    \label{fig:sdm}
% \end{figure}

One of the most widely used versions of SDM is v1.5\footnote{https://github.com/runwayml/stable-diffusion/tree/08ab4d326c96854
026c4eb3454cd3b02109ee982}. We provide the FLOPs and latency profile of SDM-v1.5 in Figs.~\ref{fig:over_flops}, \ref{fig:flops_15}, and \ref{fig:latency_15}. Fig. \ref{fig:over_flops} shows that the sampling cost dominates the image generation cost. Figs. \ref{fig:flops_15} and \ref{fig:latency_15} show that the cost of attention layers dominates the sampling cost in terms of both FLOPs and latency.

\begin{figure}[h]
  \centering
   \includegraphics[width=\linewidth]{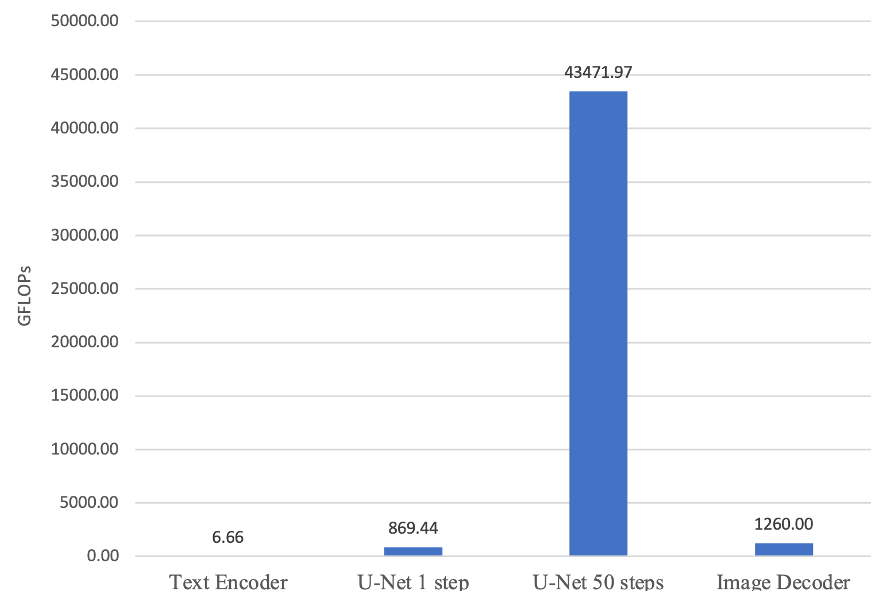}

   \caption{The FLOPs breakdown of SDM-v1.5. Measured with 512$\times$512 px image generation.}
   \label{fig:over_flops}
\end{figure}

\begin{figure}[h]
  \centering
   \includegraphics[width=\linewidth]{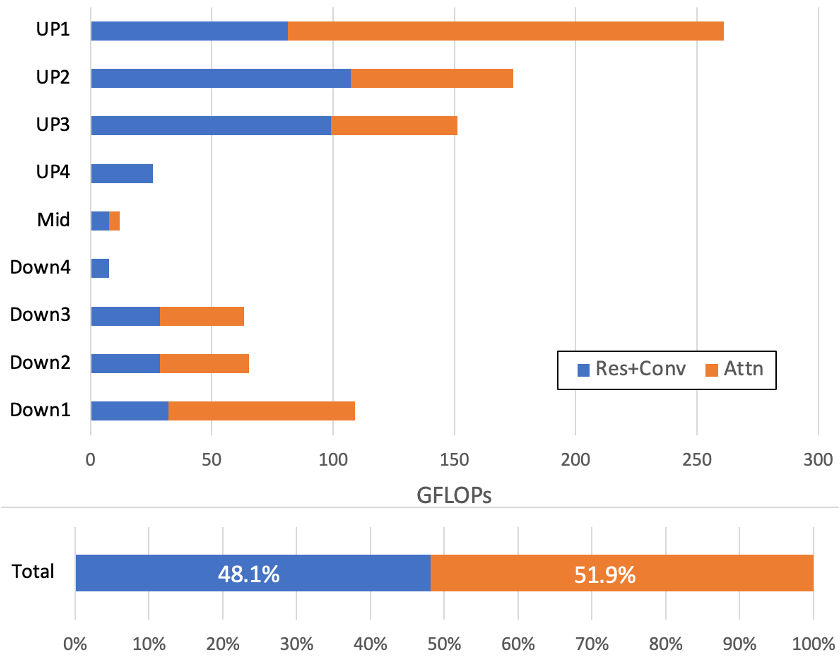}

   \caption{The FLOPs breakdown of the stages in the U-Net of SDM-v1.5. Measured with 512$\times$512 px image generation.}
   \label{fig:flops_15}
\end{figure}

\begin{figure}[h]
  \centering
   \includegraphics[width=\linewidth]{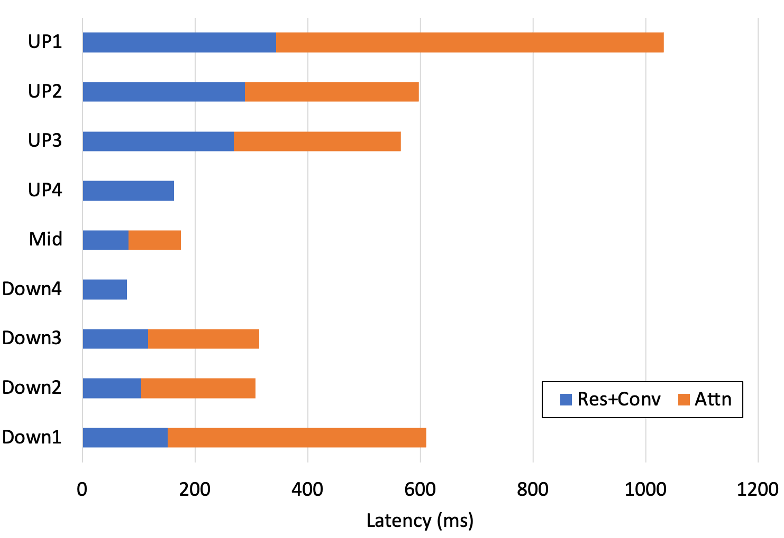}

   \caption{The latency breakdown of the stages in the U-Net of SDM-v1.5. Measured with 512$\times$512 px image generation on a single A100-40G.}
   \label{fig:latency_15}
\end{figure}

Its most powerful version is Stable Diffusion XL \cite{sdxl}. Compared with previous versions of SDM, it increases the quality of generated images significantly while maintaining similar generation latency when the resolution is higher than 768$\times$768 pixels, as shown in Fig.~\ref{fig:comp_sd}. Thus, we select SD-XL as the default backbone in our work. In SD-XL, attention blocks at the highest level are removed and the number of attention blocks at the lowest abstraction level increased by 10$\times$. Its FLOPs, latency, and parameters profiles are shown in Figs.~\ref{fig:flops_xl}, \ref{fig:latency_xl}, and \ref{fig:param_xl}, respectively. We observe that attention blocks still dominate the computational cost in the new architecture.

\begin{figure}[h]
  \centering
   \includegraphics[width=\linewidth]{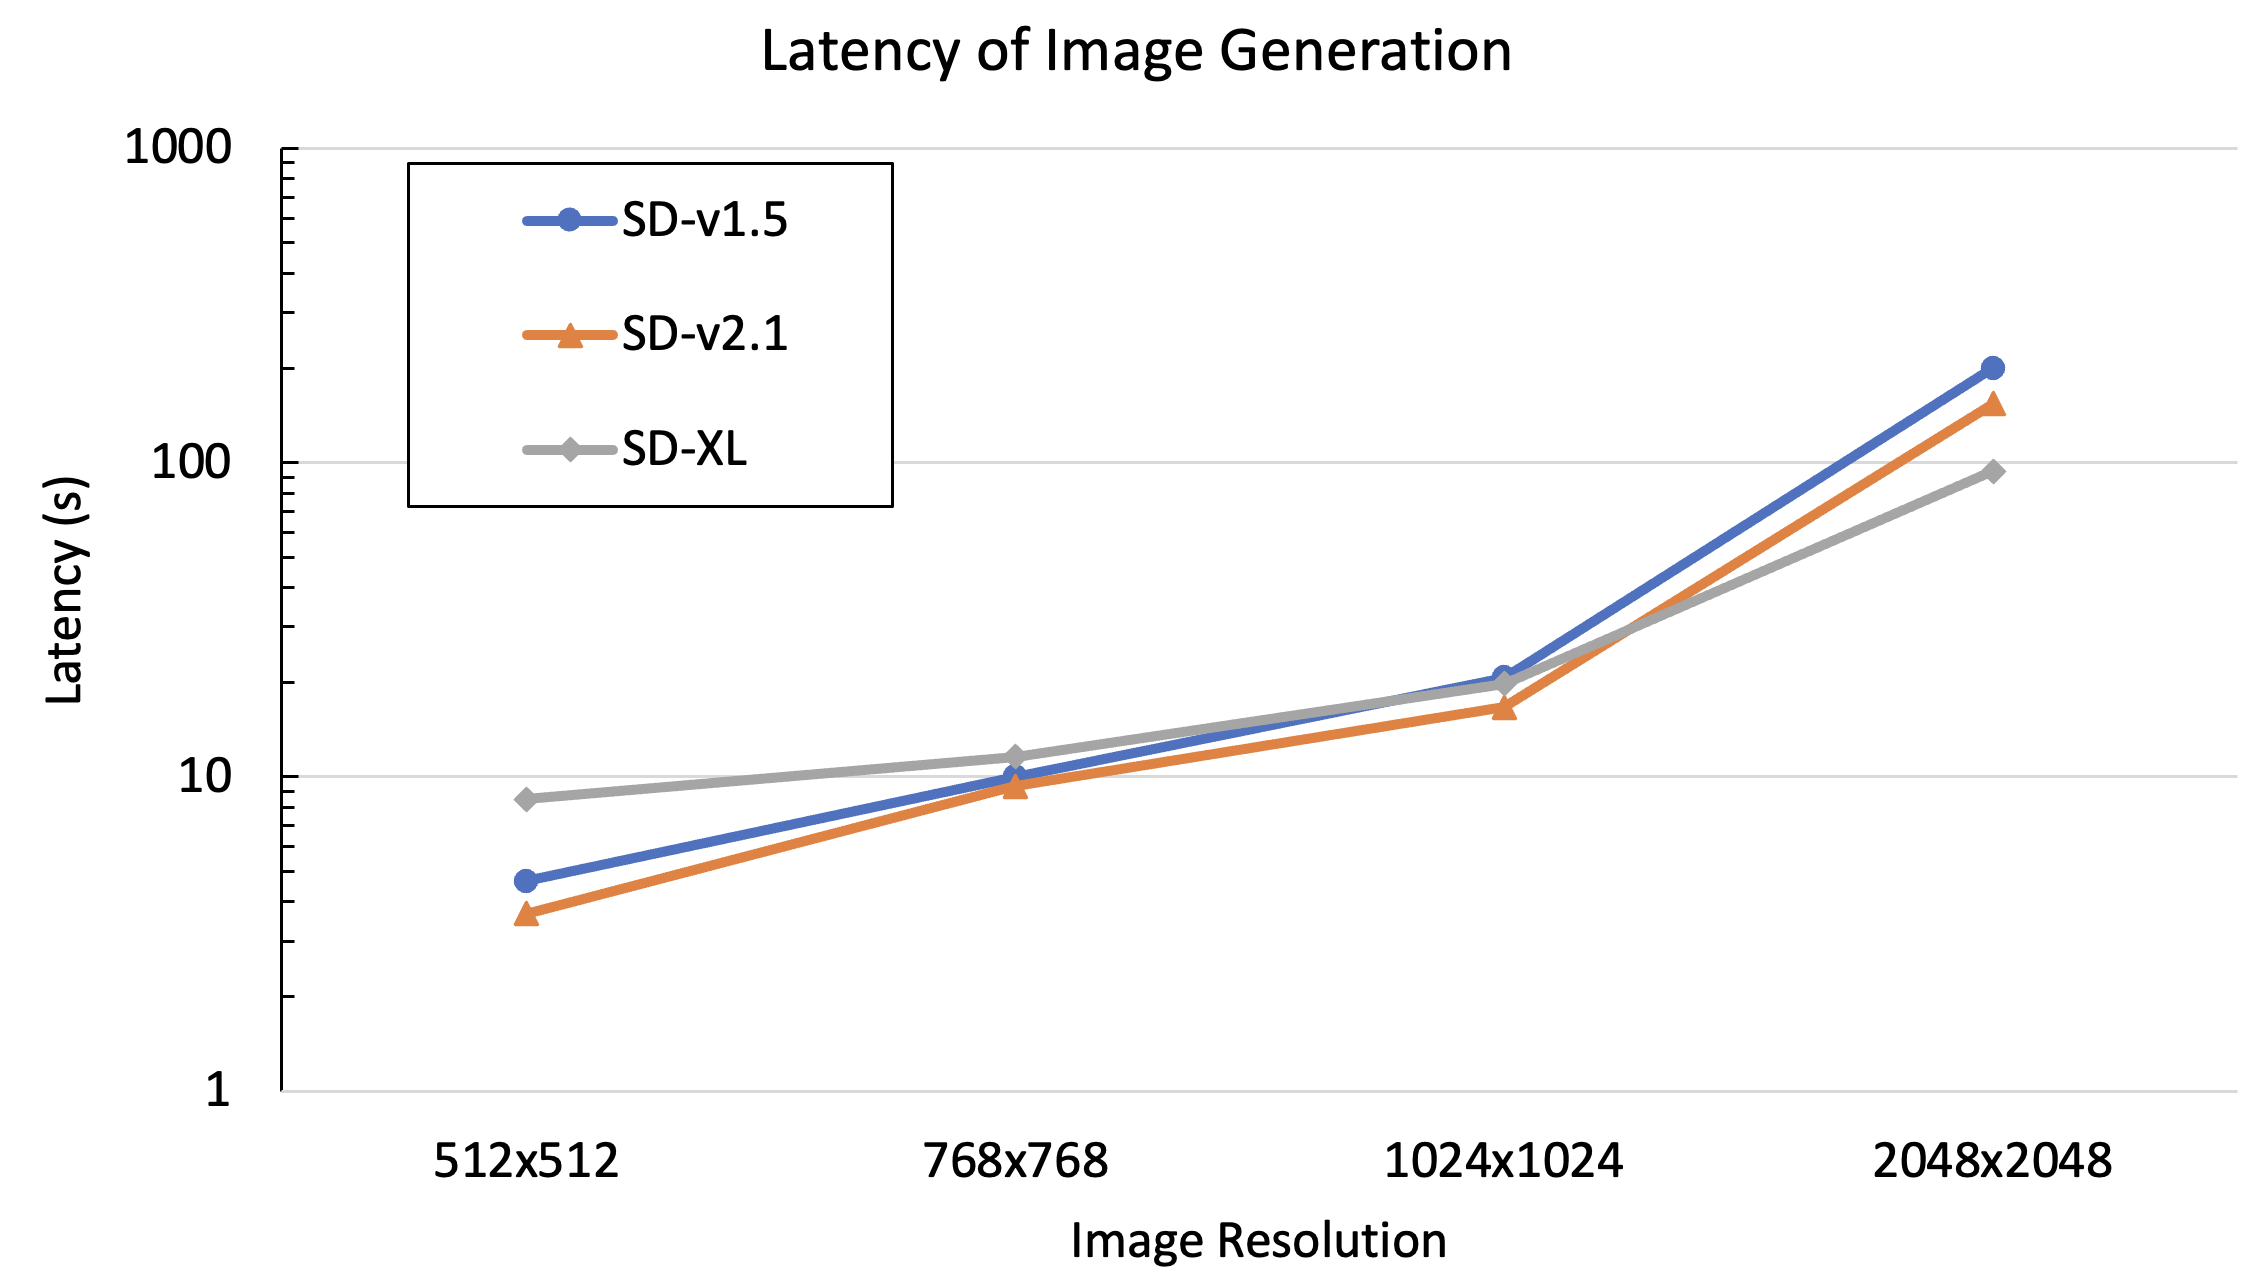}

   \caption{Image generation latency comparison among different models at different resolutions. When the resolution equals or is higher than 1024$\times$1024, SD-XL has an even lower latency than SD-v1.5 and SD-v2.1, despite much higher image quality.}
   \label{fig:comp_sd}
\end{figure}

\begin{figure}[h]
  \centering
   \includegraphics[width=\linewidth]{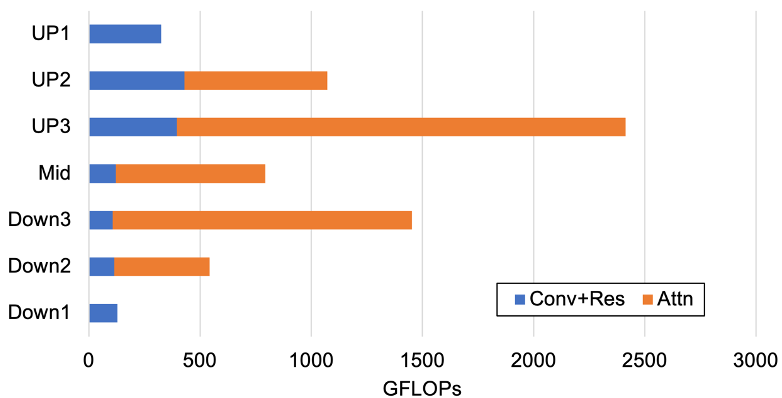}

   \caption{The FLOPs breakdown of SD-XL. Measured with 1024$\times$1024 px image generation.}
   \label{fig:flops_xl}
\end{figure}

\begin{figure}[h]
  \centering
   \includegraphics[width=\linewidth]{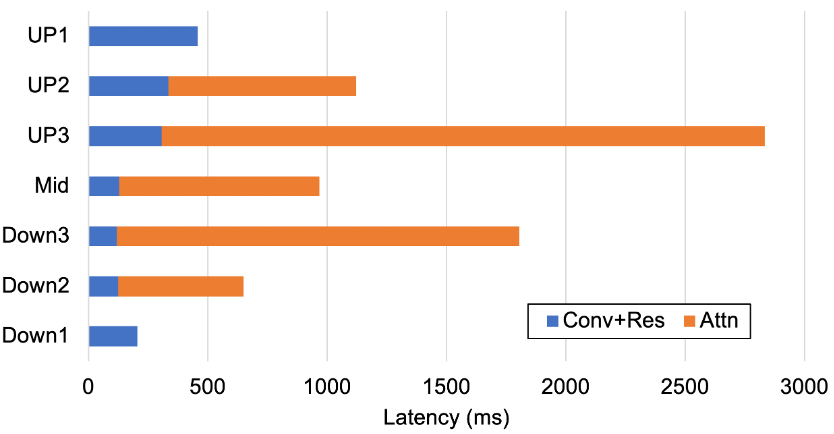}

   \caption{The latency breakdown of SD-XL. Measured with 1024$\times$1024 px image generation on a single A100-40G. The batch size is 1.}
   \label{fig:latency_xl}
\end{figure}

\begin{figure}[h]
  \centering
   \includegraphics[width=\linewidth]{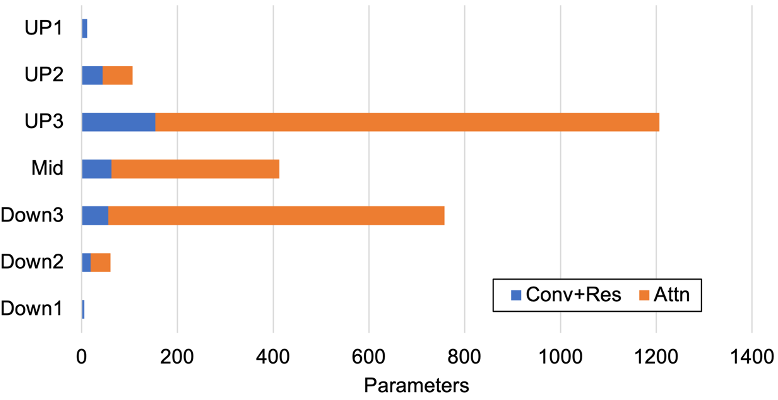}

   \caption{The parameters breakdown of SD-XL. Measured with 1024$\times$1024 px image generation.}
   \label{fig:param_xl}
\end{figure}

We also investigate the scaling law of SD-XL at different generation resolutions. Fig.~\ref{fig:sdxl_scale_la} shows the latency breakdown of SD-XL at different image resolutions. The latency ratio between ResNet blocks and attention blocks is nearly constant across different resolutions, as shown in Fig. \ref{fig:sdxl_scale_ratio_la}. In SD-XL, the FLOPs of attention blocks do not scale much faster than the FLOPs of ResNet blocks when the generation resolution increases, as shown in Fig. \ref{fig:sdxl_scale_ratio_flop}. This behavior is different from what is exhibited by previous versions of SDM (shown in Fig. \ref{fig:tome_latency_ratio}). We believe this is due to the elimination of attention blocks at the highest level and the addition of attention layers at the lowest abstraction level, making the cost of feed-forward layers, which scales linearly with an increment in token numbers, a huge part of the cost of attention layers.

\begin{figure}[h]
  \centering
   \includegraphics[width=\linewidth]{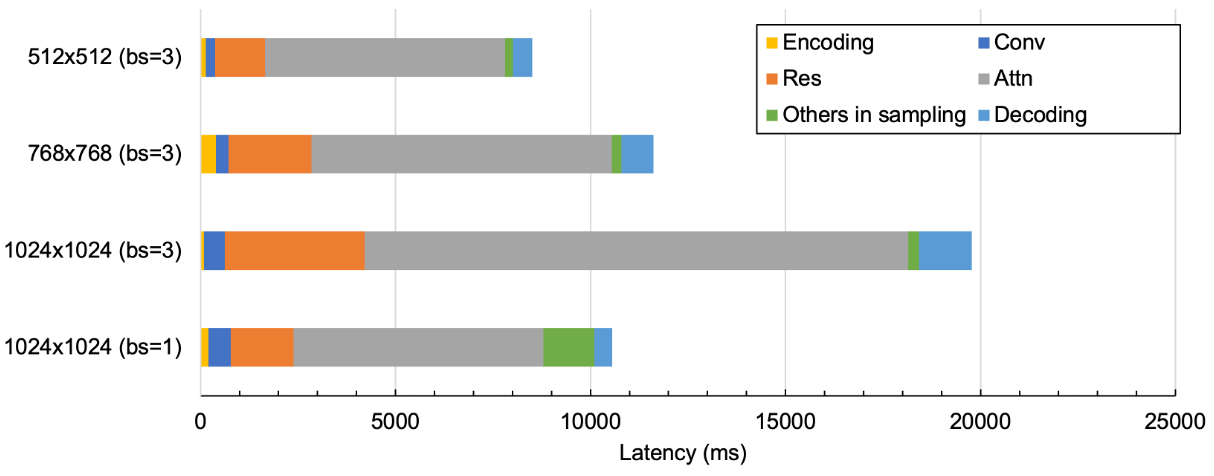}
   \caption{The latency breakdown of SD-XL at different image resolutions. ``bs" is short for ``batch size". Latency is measured on a single A100-40G.}
   \label{fig:sdxl_scale_la}
\end{figure}

\begin{figure}[h]
  \centering
   \includegraphics[width=\linewidth]{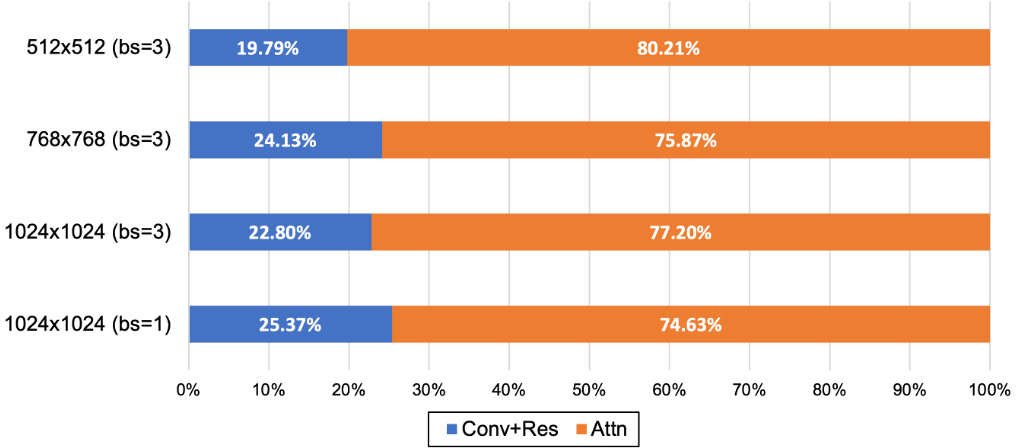}
   \caption{The latency ratio between ResNet blocks and attention blocks of SD-XL at different image resolutions. ``bs" is short for ``batch size". Latency is measured on a single A100-40G.}
   \label{fig:sdxl_scale_ratio_la}
\end{figure}

\begin{figure}[h]
  \centering
   \includegraphics[width=\linewidth]{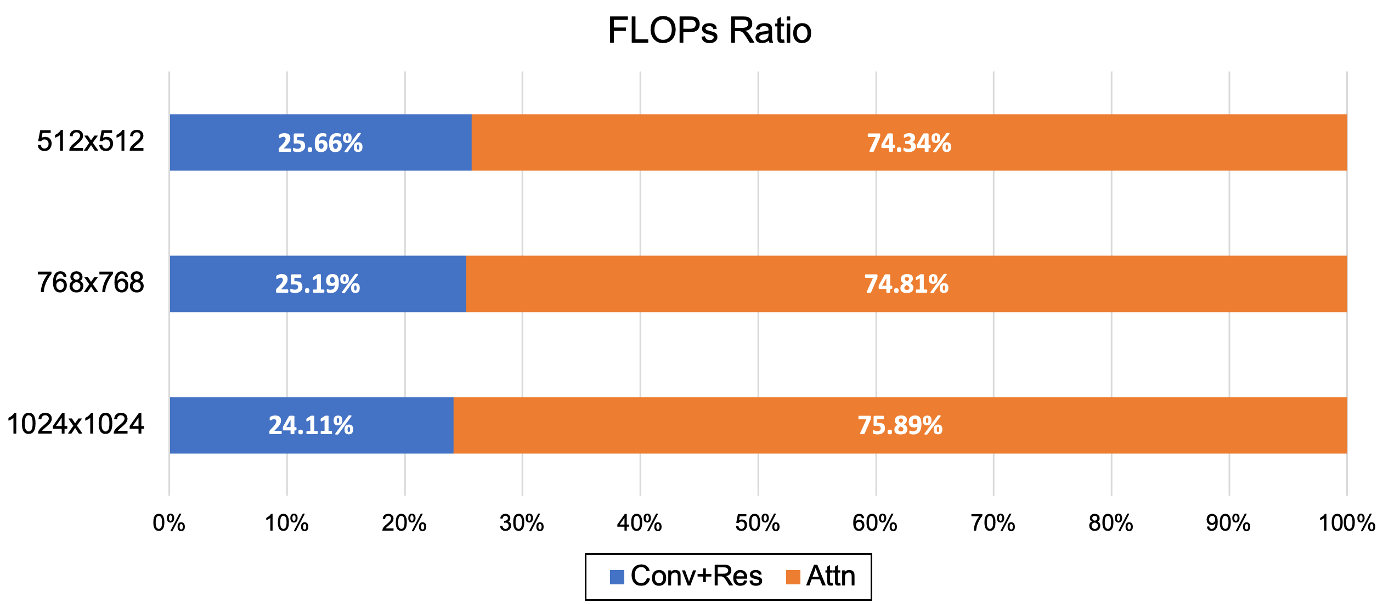}
   \caption{The FLOPs ratio between ResNet blocks and attention blocks of SD-XL at different image resolutions. ``bs" is short for ``batch size".}
   \label{fig:sdxl_scale_ratio_flop}
\end{figure}

\subsection{Token Merging}

Most previous works require retraining of the DM backbone to enhance efficiency, which usually requires thousands of A100 GPU hours. 
%The cost is not only expensive for personal users and researchers at universities, but also expensive for companies in the industry. 
Because it is not a once-for-all method and scales with model size, a training-free method to enhance the efficiency of DMs is needed.

 Token Merging (ToMe) \cite{tomesd} is a training-free pruning method. It merges similar tokens before self-attention, cross-attention, and feed-forward network and unmerges tokens back after that. Note that it only reduces the cost of attention blocks in the U-Net. This is reasonable because for $N\times N$ pixels image generation, the computational overhead of ResNet blocks scales as $O(N^2)$; however, the overhead of attention blocks scales as $O(N^4)$.

\begin{figure}[t]
  \centering
   \includegraphics[width=\linewidth]{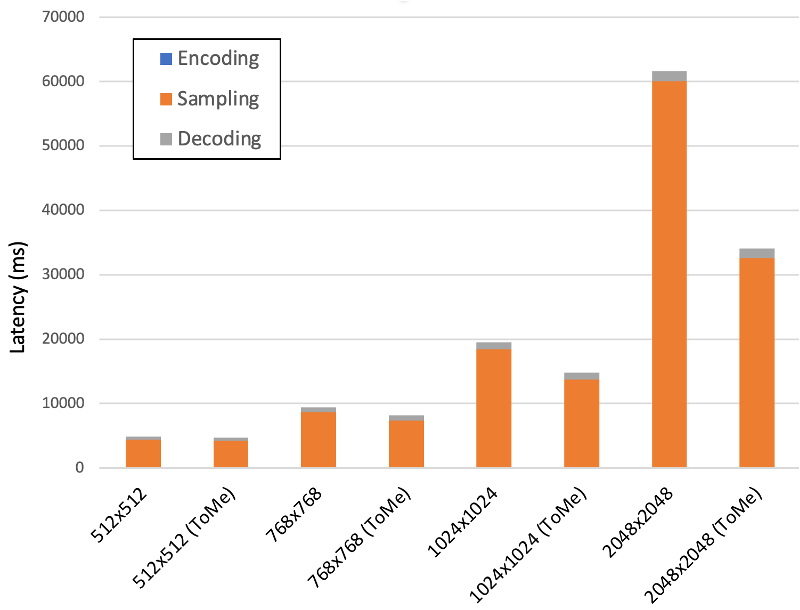}
   \caption{The latency breakdown before and after ToMe is applied to SD-v1.5. ToMe only results in a marginal speed-up when resolution is lower than 1024$\times$1024 px. Latency is measured on a single A100-40G.}
   \label{fig:tome_latency}
\end{figure}

\begin{figure}[t]
  \centering
   \includegraphics[width=\linewidth]{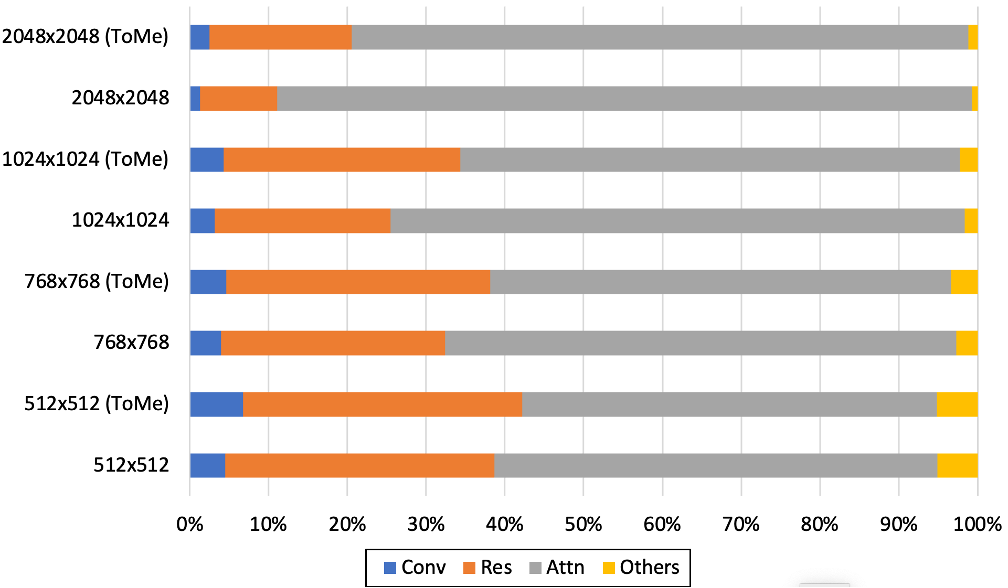}
   \caption{The latency proportion of sampling before and after ToMe is applied to SD-v1.5 at different image resolutions. As the resolution increases, the proportion of attention layers increases significantly. Latency is measured on a single A100-40G.}
   \label{fig:tome_latency_ratio}
\end{figure}

As shown in Fig.~\ref{fig:tome_latency_ratio}, in SD-v1.5, the latency proportion of attention layers increases significantly as the resolution increases for image generation. Thus, ToMe only results in a marginal speed-up when the resolution is lower than 1024$\times$1024 px.

When ToMe is applied to a state-of-the-art backbone, SD-XL, the results degrade further. Since SD-XL eliminates attention layers at the highest abstraction level, native ToMe does not do anything to this backbone (it only merges tokens for attention layers at the highest abstraction level). Thus, we expand its merging range to all attention layers, including self-attention, cross-attention, and feed-forward layers in them. Although this setting reduces FLOPs a lot, it results in only a marginal speed-up in latency, as shown in Fig.~\ref{fig:tome_save}. This is not because the merging rate is too low. If we randomly drop the same number of tokens, the speed-up is much more significant. We believe the actual reason is that the token merging algorithm is too costly, with a complexity of $O(N^2\times d)$, where $N$ is the number of tokens and $d$ is the dimension of token embeddings. Both are usually larger than 1000. Given the huge quality degradation caused by ToMe (see Section \ref{sec:experiments}), its use is not recommended with SD-XL.

\textbf{Needs to modify} It is even more worrisome that such a huge quality decay is not exchanged for significant speed-up. Based on our experiments on a single NVIDIA A100-40GB GPU, ToMe reduces latency by only 3\%. This is not due to the fact that the number of reduced tokens is not enough. If we drop the same number of tokens randomly, the latency can be reduced by more than 28\%. Thus, we believe the actual reason is that ToMe's token merging algorithm is too complex. ToMe's token merging algorithm has a complexity of $O(N^2\times d)$, where $N$ is the number of tokens and $d$ is the dimension of token embeddings. Both are typically larger than 1000. For comparison, the complexity of our WPR algorithm is $O(N^2)$.

\begin{figure}[t]
  \centering
   \includegraphics[width=\linewidth]{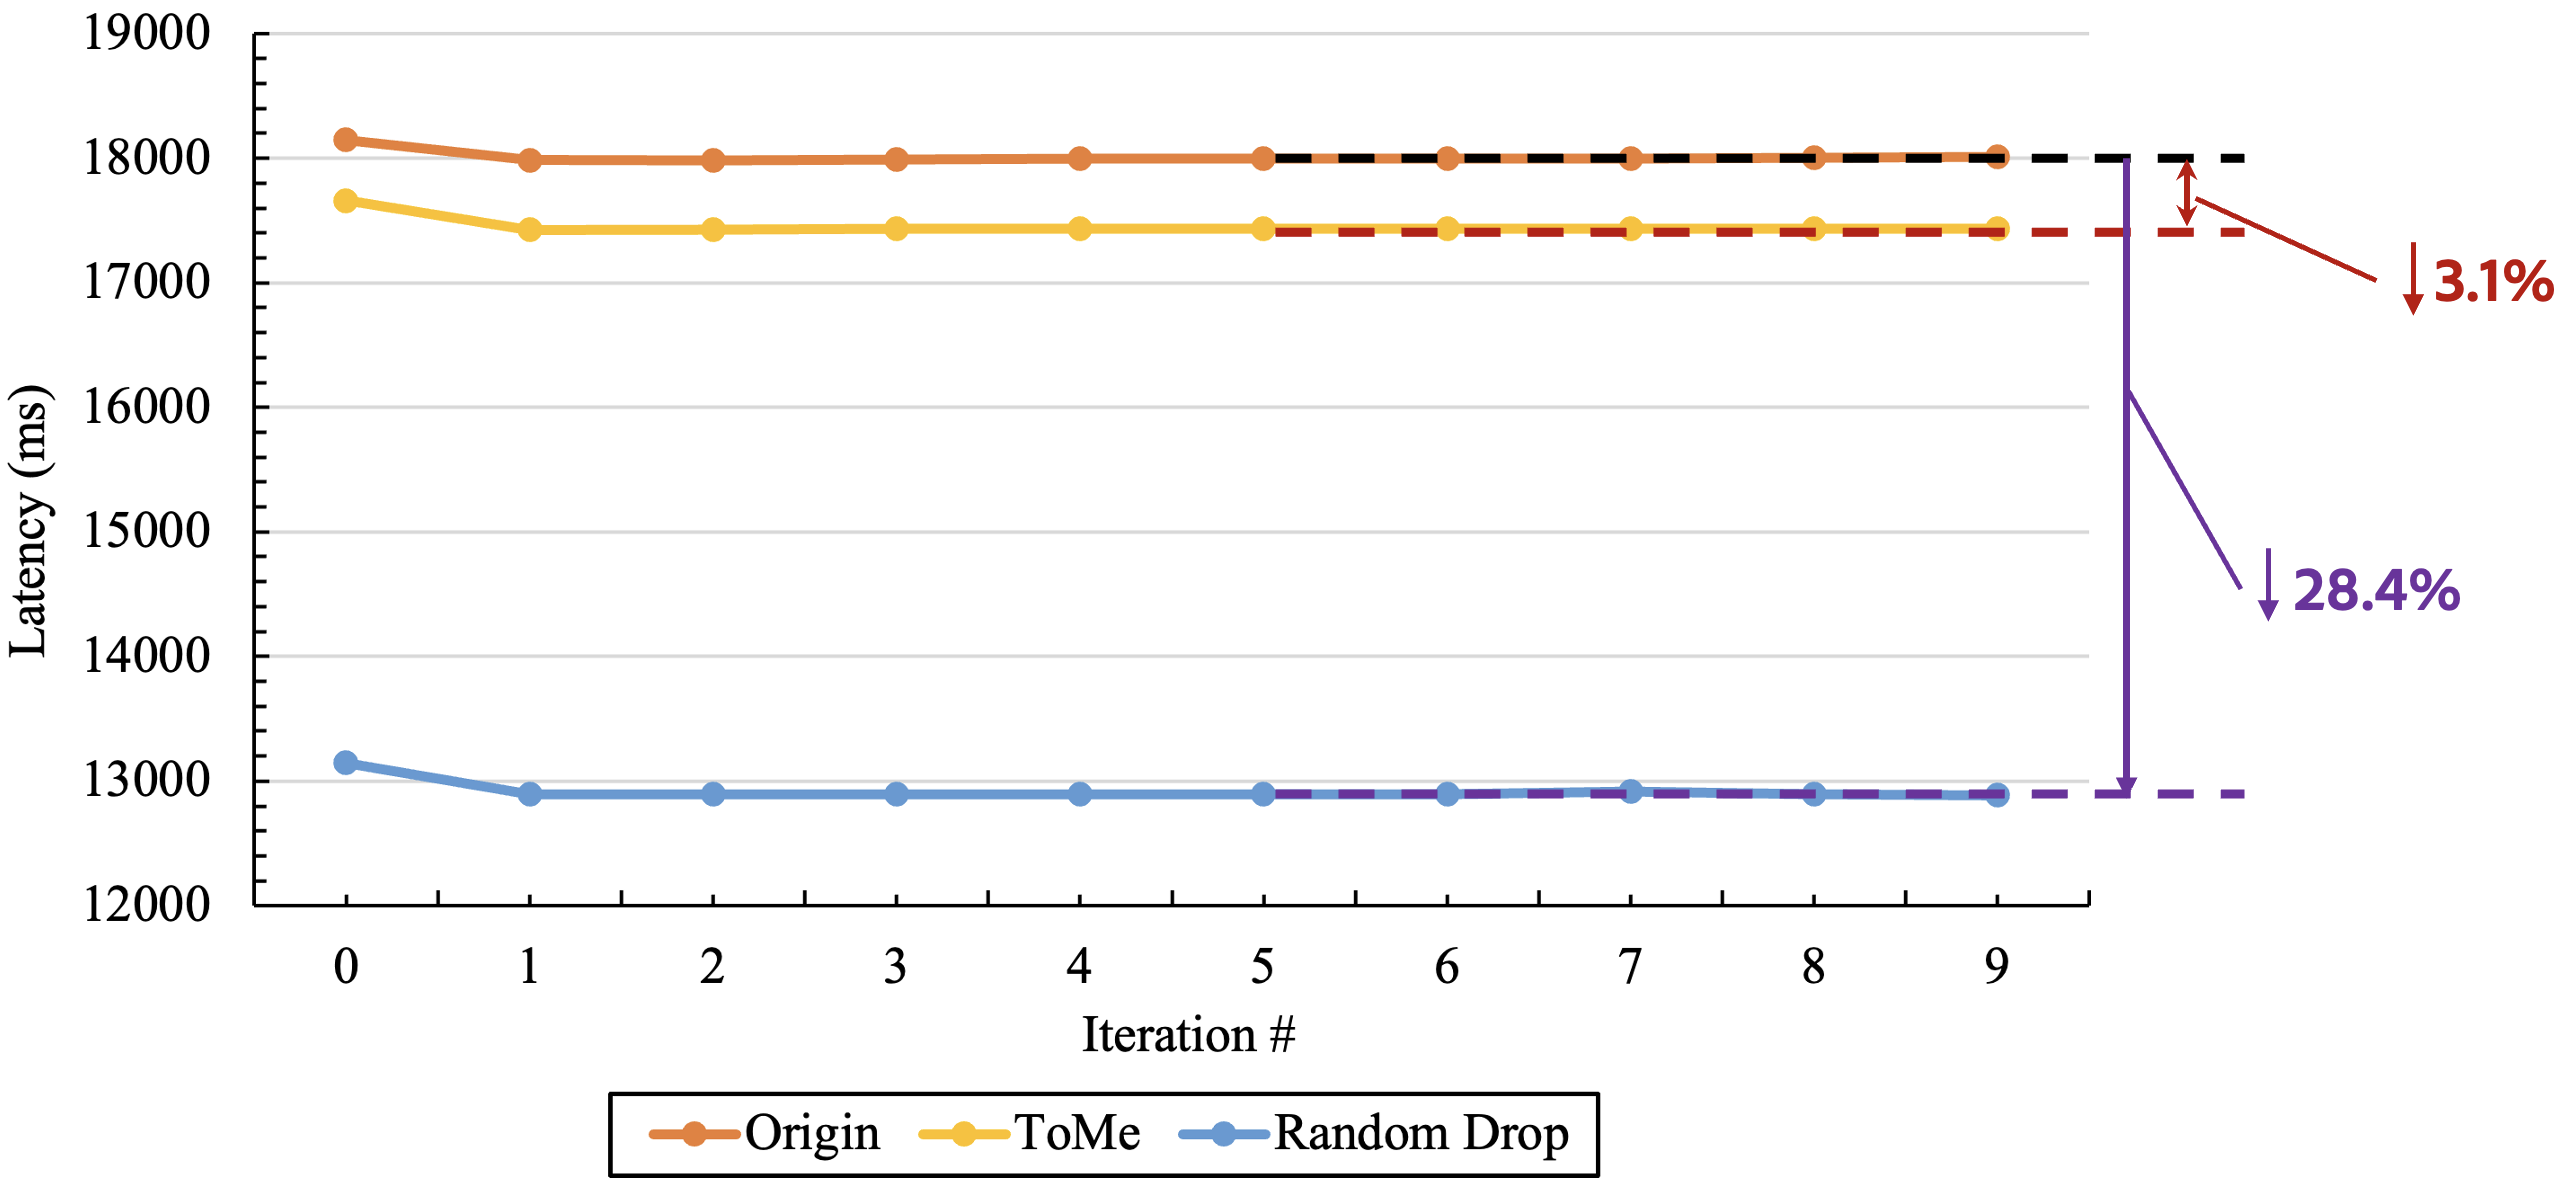}
   \caption{Speed-up of ToMe and randomly dropping the same number of tokens. Speed-up is obtained by averaging the latency over nine iterations (the first iteration is eliminated due to GPU warm-up).}
   \label{fig:tome_save}
\end{figure}

\section{Location of Deploying Run-Time Pruning}

In our default setting, we use generated masks after the feed-forward layer to perform token pruning. Another option is performing pruning early before the feed-forward layers, which brings extra FLOP savings at the cost of image quality.

\section{Implementations of CA-based WPR}

To generalize WPR to cross-attention, we need to design a function $f(\mathbf{A},s_K)$ that maps the importance of Key tokens to that of Query tokens. The intuition of designing this function is that vital Query tokens should devote much of their attention to important Key tokens. Thus, the desired attention distribution should satisfy: (1) 

\section{Heterogeneous Sampling}

In AT-EDM, we design a cross-step pruning schedule that is less aggressive for early denoising steps. In this section, we first provide experimental results of pruning more in early denoising steps to justify our choice and then provide a detailed description of our less aggressive pruning schedule in early steps.

\subsection{Prune More in Early Denoising Steps}

\subsection{Less Aggressive Pruning Schedule}
\label{app:lessprune}

Early denoising steps determine the layout of the generated images and have weaker ability to differentiate between unimportant tokens \cite{prompt2prompt}. Thus, we need heterogeneous denoising steps and, hence, use a less aggressive pruning schedule for some of the early denoising steps. The U-Net architecture of SD-XL and the design of the less-aggresive pruning schedule are shown in Fig.~\ref{fig:sdxl_unet}.

\begin{figure}[h]
  \centering
   \includegraphics[width=\linewidth]{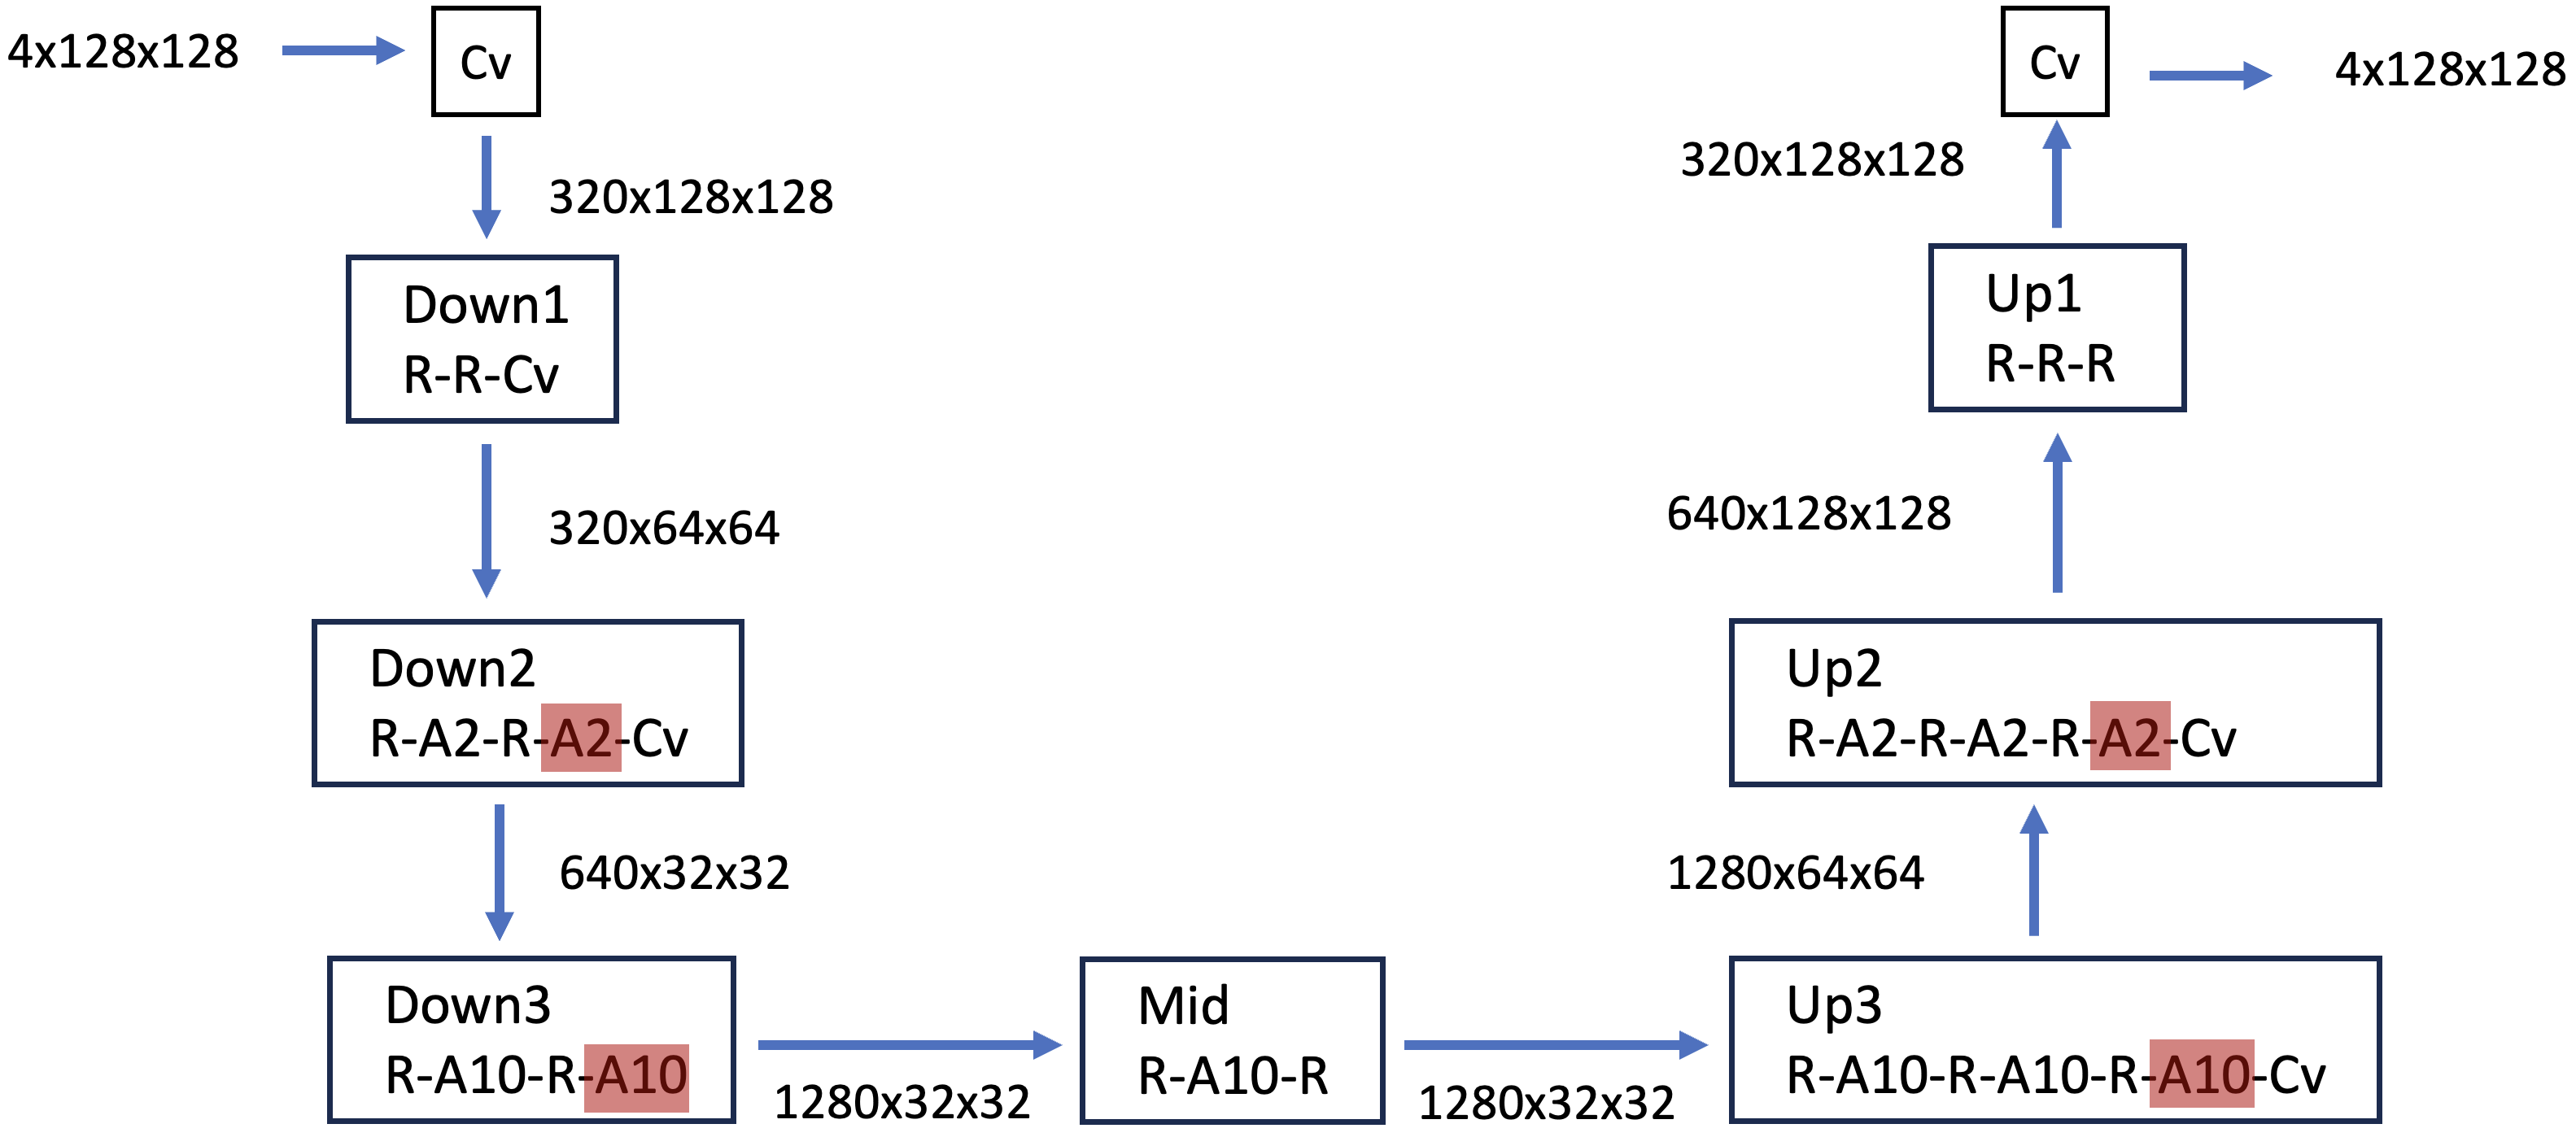}
   \caption{The U-Net architecture of SD-XL. A2 represents an attention block that includes two attention layers; A10 represents an attention block that includes 10 attention layers. The example in this figure generates a 1024$\times$1024 pixels image. In the less-aggressive pruning schedule, we do not apply pruning to attention blocks in the red rectangles.}
   \label{fig:sdxl_unet}
\end{figure}

In the normal pruning setting, when we target 4.1 TFLOPs for each sampling step, we use a pruning rate of 60\% (i.e., retain 40\% tokens) after the first attention layer of A2 and A10; for the less-aggressive pruning schedule, we do not apply pruning to attention blocks in the red rectangles, as shown in Fig. \ref{fig:sdxl_unet}. This is based on the intuition that attention blocks at the end of up/down-stages are more important than other attention blocks. 



% \section{More Visual Examples}
% \label{app:visual}

% \label{sec:rationale}
% % 
% Having the supplementary compiled together with the main paper means that:
% % 
% \begin{itemize}
% \item The supplementary can back-reference sections of the main paper, for example, we can refer to \cref{sec:intro};
% \item The main paper can forward reference sub-sections within the supplementary explicitly (e.g. referring to a particular experiment); 
% \item When submitted to arXiv, the supplementary will already included at the end of the paper.
% \end{itemize}
% % 
% To split the supplementary pages from the main paper, you can use \href{https://support.apple.com/en-ca/guide/preview/prvw11793/mac#:~:text=Delete%20a%20page%20from%20a,or%20choose%20Edit%20%3E%20Delete).}{Preview (on macOS)}, \href{https://www.adobe.com/acrobat/how-to/delete-pages-from-pdf.html#:~:text=Choose%20%E2%80%9CTools%E2%80%9D%20%3E%20%E2%80%9COrganize,or%20pages%20from%20the%20file.}{Adobe Acrobat} (on all OSs), as well as \href{https://superuser.com/questions/517986/is-it-possible-to-delete-some-pages-of-a-pdf-document}{command line tools}.

\section{Pruning with Various FLOPs Budgets}

\subsection{Visual Examples for comparison}

\subsection{FID-CLIP Scores}

\section{Calibration Block for FLOPs Measurement}

\section{More Images from AT-EDM and ToMe}

\section{Deploying ToMe on SD-XL}

For former versions of Stable Diffusion Models, such as SD-v1.5 and SD-v2.1, ToMe \cite{tomesd} maintains the image quality well with the default setting after ToMe Merging. In the default setting of ToMe, ToMe only applies token merging to the down-stage and up-stage with the highest resolution. However, SD-XL deletes the attention block in these stages, incurring the default setting of ToMe cannot bring any FLOPs savings.
